# Supplementary material for: Work-distribution quantumness and irreversibility when crossing a quantum phase transition in finite time
Source: arXiv:1908.06488 source file (2019-08-28)
Supplement: Supplementary file 1 [file supplemental_material.pdf]

# Supplemental Material – Work-distribution quantumness and irreversibility when crossing a quantum phase transition in finite time

Krissia Zawadzki,[1,2] Roberto M. Serra,[3] and Irene D'Amico[4,1,5]

[1] *Departamento de Física e Ciência Interdisciplinar, Instituto de Física de São Carlos, University of São Paulo, Caixa Postal 369, 13560-970 São Carlos, SP, Brazil*
[2] *Department of Physics, Northeastern University, Boston, Massachusetts 02115, USA*
[3] *Centro de Ciências Naturais e Humanas, Universidade Federal do ABC, Avenida dos Estados 5001, 09210-580, SantoAndré, São Paulo, Brazil*
[4] *Department of Physics, University of York, York, YO10 5DD, United Kingdom*
[5] *International Institute of Physics, Federal University of Rio Grande do Norte, Natal, Brazil*

## Evolution of work probability distribution

In our letter, we presented 3-dimensional plots for the evolution of the work probability distributions $P(W)$ with respect to the driving time $\tau$, for chains of sizes $L = 4$ and $L = 8$ within zero and strong-coupling regimes, $U = 0J$ and $U = 10J$ respectively.

Here, we provide animations showing $P(W)$ evolving with $\tau$, $\tau J = 0.2, ..., 1.0, 1.5, 2.0, ..., 10.0$, for fixed value of $U$ ($U/J = 0.0, 1.0, 2.0, ..., 10.0$) and for all the considered chain lengths, $2 \leq L \leq 8$. The animations clearly show how the distribution is strongly $\tau$-dependent below the pM-QPT (weak many-body correlations), to become basically $\tau$-independent above the pM-QPT (strong many-body correlations). These animations are available in the Figs named work_distribution_beta=0.4_L=NSITES_U=COULOMB.gif, with NSITES=2,4,6,8 and COULOMB varying according to the range $U/J$ above.

## Moments of the quantum work probability distribution

As discussed in our letter, the statistics of the quantum work distribution $P(W)$ can be characterized by its momenta. Of particular importance are: its average $\langle W \rangle$; standard deviation $\langle W - \bar{W} \rangle^2$; and skewness, or third central momentum $\langle W - \bar{W} \rangle^3$. Here we present the heatmaps of these quantities – and in addition of the curtosis, or fourth central momentum $\langle W - \bar{W} \rangle^4$ – with respect to $U$ and $\tau$, and for all considered system sizes $L = 2,\ 4,\ 6,\ 8$, see Figs. 1–4. To facilitate the comparison, we include here also the skewness for $L = 4$ and $L = 8$, already presented in the main text.

The heatmaps of the work produced by applying the external electric field is shown in panel (a) of Figs. 1–4, for $0 \leq U \leq 10J$ and $0.2/J \leq \tau \leq 10$. The freezing of the system due to the pM-QPT results in a dramatic reduction in the extractable work for all values of $L$.

For $L = 4,\ 6,\ 8$ the first four momenta of $P(W)$ display a *qualitative* behaviour which is size-independent, with the white lines in the heatmaps for the skewness $k = 3$ representing the points at which this quantity is zero. Also, for the same $L$, standard deviation and curtosis have qualitatively similar behaviours.

However, for $L = 2$, the skewness remains negative for all coupling regimes $U$ and driving times $\tau$, while the curtosis displays a behaviour qualitatively different from the standard deviation for weak interactions and intermediate to long driving times.

## Entropy production

The entropy production corresponding to the average quantum work produced for $L = 4$ and $L = 8$ is plotted in Fig. 5, left and right panel, respectively. For low-correlations the entropy is strongly sensitive to the dynamical regime, and decreases as the system becomes more adiabatic. Note that, for a finite quantum system, adiabaticity does not imply equilibration, so the entropy is expected to remain finite for increasing $\tau$. At high correlations, the entropy remains relatively low independently of $\tau$.

The overall entropy behavior implies that, for the same type of driving potential and same driving time, tailoring many-body interactions may be used to approach – or not – equilibrium.

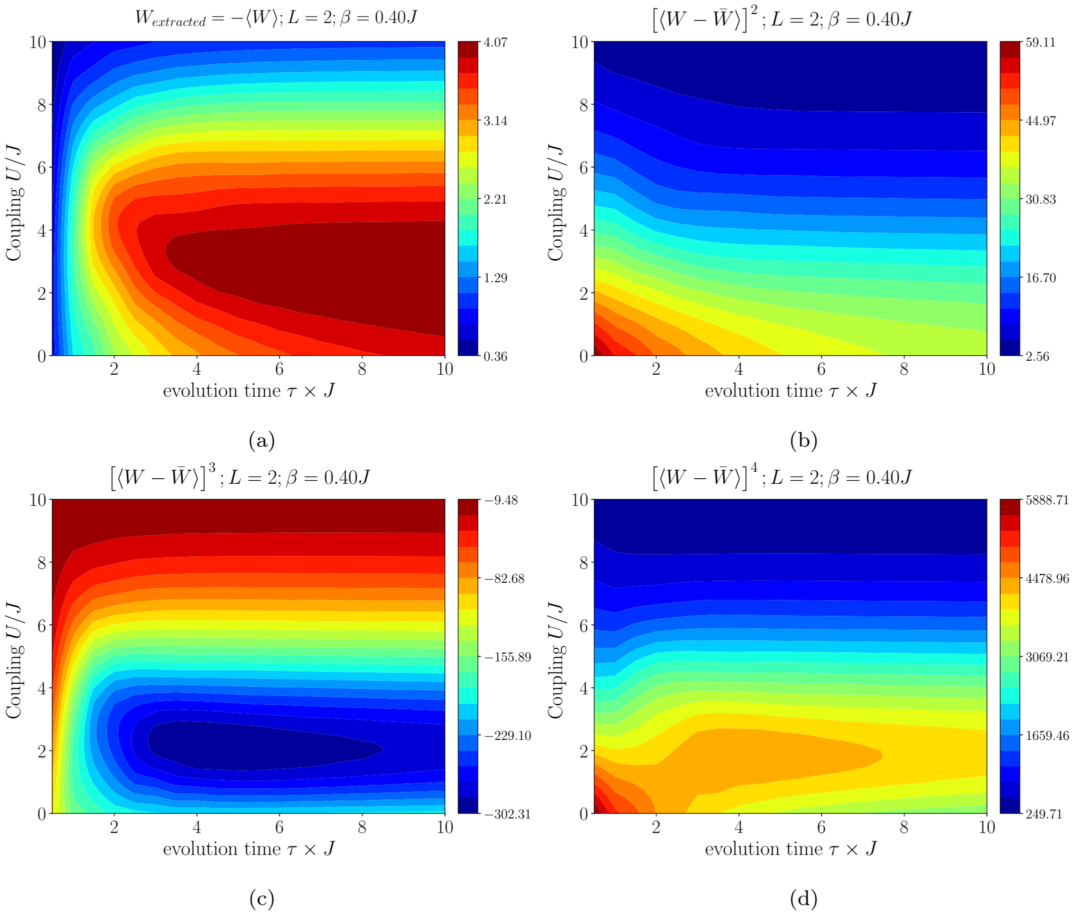


Figure 1: Heatmaps of the average work and the following three central momenta $\langle W - \bar{W} \rangle^k$ $k = 2, 3, 4$ for $L = 2$.

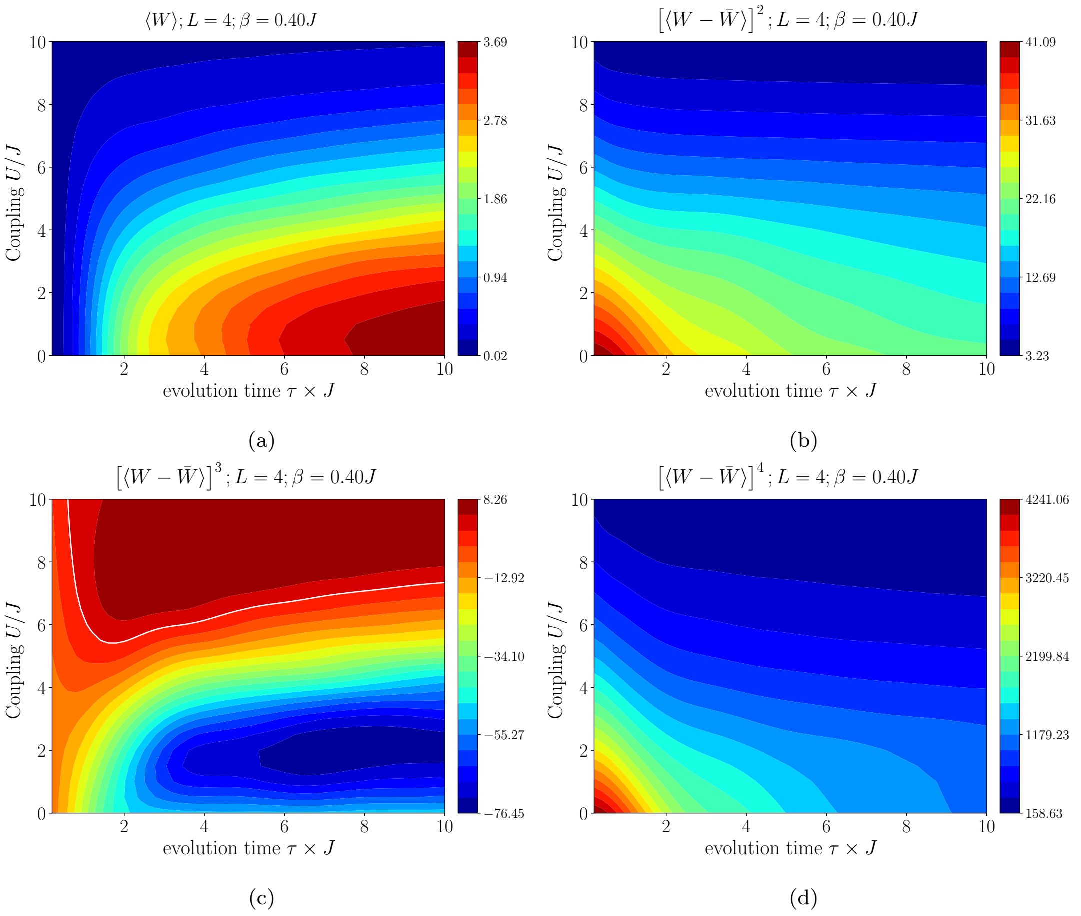


Figure 2: Heatmaps of the average work and the following three central momenta $\langle W - \bar{W} \rangle^k$ $k = 2, 3, 4$ for $L = 4$.

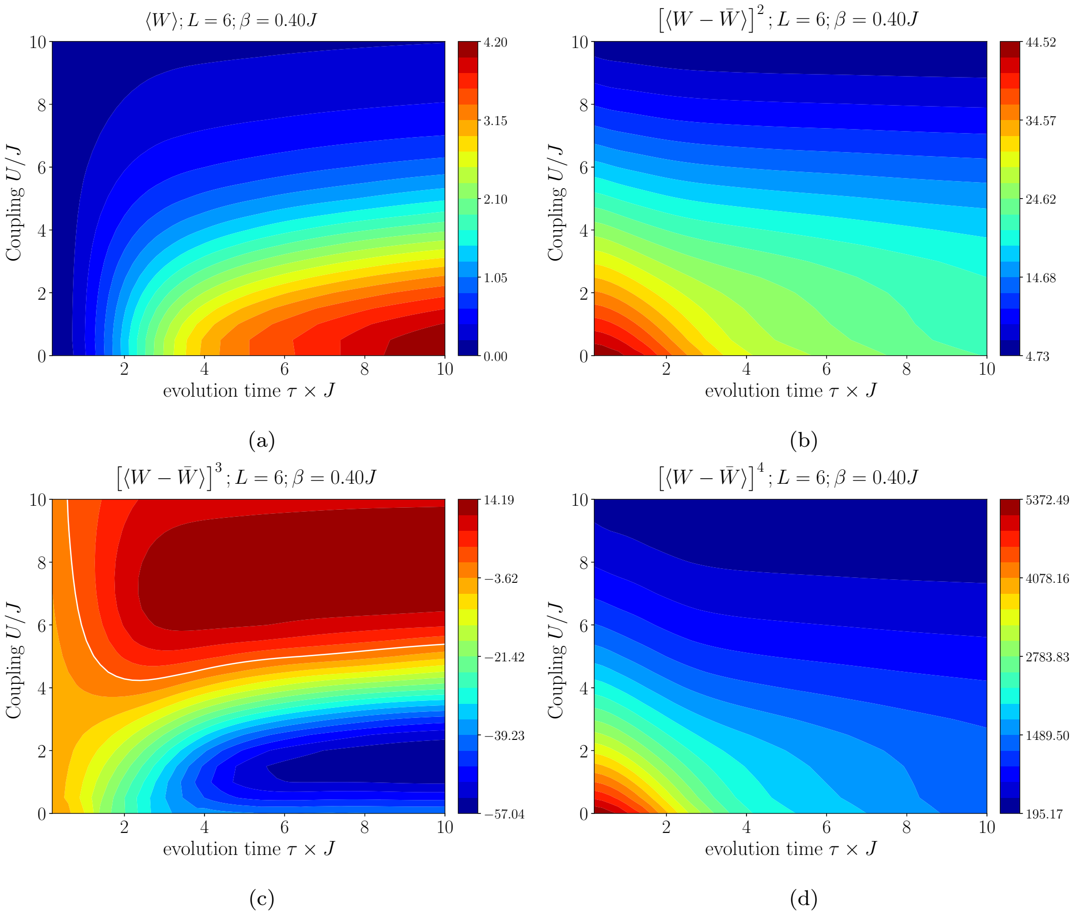


Figure 3: Heatmaps of the average work and the following three central momenta $\langle W-\bar{W}\rangle^k$ $k=2,3,4$ for $L=6$.

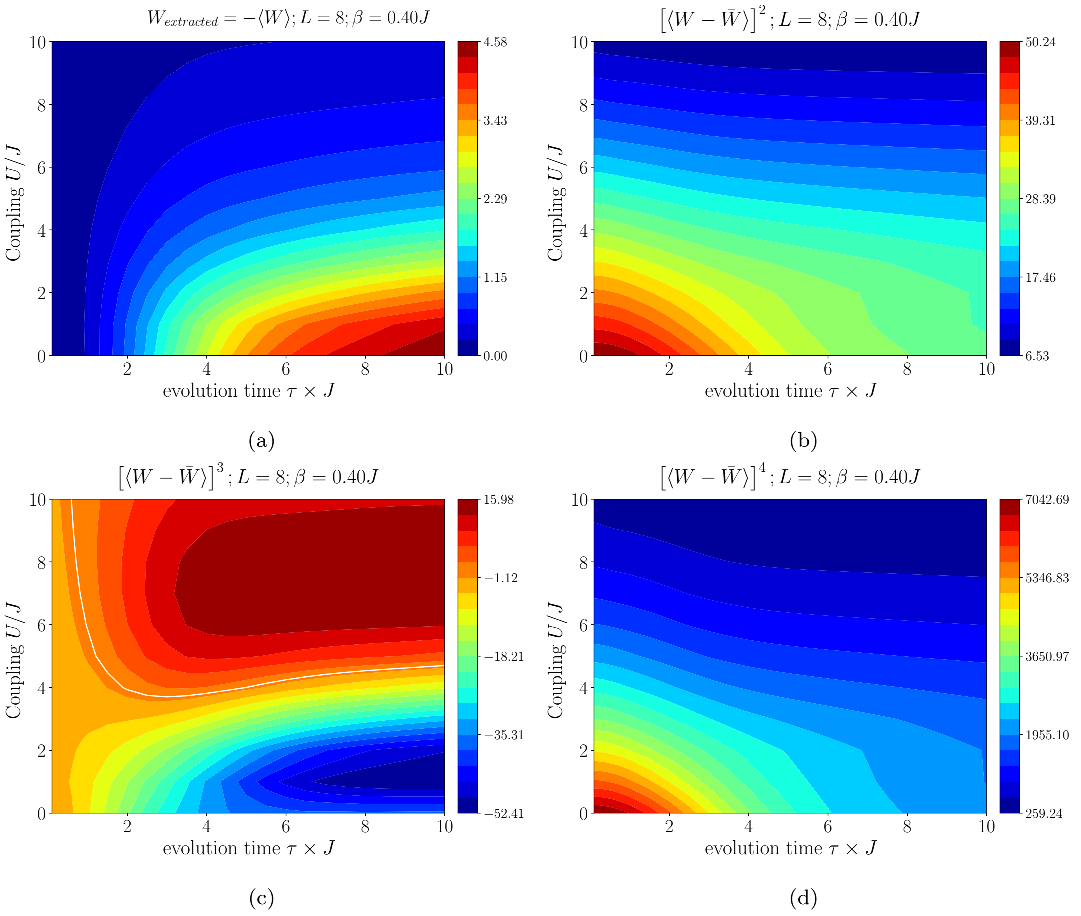


Figure 4: Heatmaps of the average work and the following three central momenta $\langle W-\bar{W}\rangle^k$ $k=2,3,4$ for $L=8$.

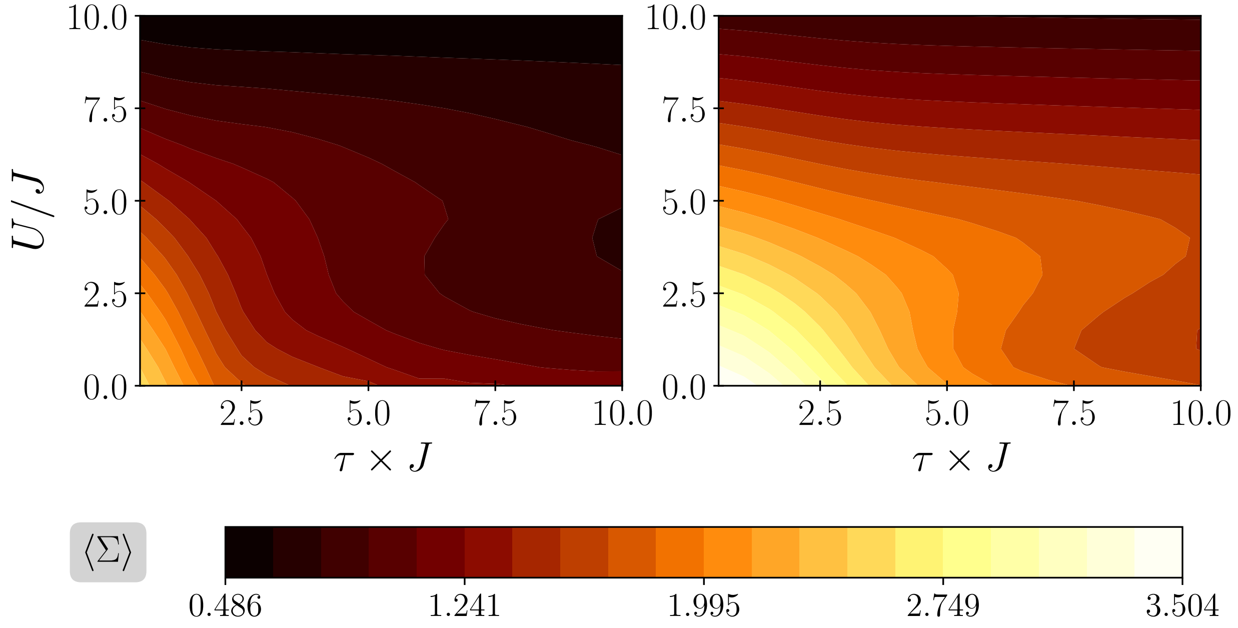


Figure 5: Heatmaps of the entropy production, for $L = 4$ (left) and $L = 8$ (right).
